# Supplementary material for: Monitoring the Economy in Real Time: Trends and Gaps in Real Activity and Prices
Source: arXiv:2201.05556 source file (2023-03-31)
Supplement: Supplementary file 1 [file appendix.tex]

\begin{appendices}

\section{Data}\label{data}

\subsection{GDP SPF}

The Survey of Professional Forecasters includes expectations for real GDP in levels and growth rates. We decided not to use the official release for the expectation of real GDP in levels, because it is not adjusted for changes in the basis year, data revisions and in the seasonal adjustment mechanism. 

Instead, we computed the one-year ahead SPF expectation for the growth rates and we used it jointly with the latest vintage of data available for real GDP to compute an adjusted prediction for the levels.

%\clearpage
\section{Adaptive Metropolis-Within-Gibbs}

\subsection{Algorithm}
\label{AMWG}

The estimation algorithm is an improved version of the Metropolis-Within-Gibbs in \cite{hasenzagl2018model} that employs the Single Component Adaptive Metropolis proposed in \cite{haario2005componentwise}. 

This hybrid algorithm is structured in two blocks: (1) a Single Component Adaptive Metropolis \citep{haario2005componentwise} step for the estimation of the state-space parameters, (2) a Gibbs sampler \citep{koopman2000fast, jarocinski2015note} to draw the unobserved states conditional on the model parameters. Since we have non-stationary unobserved states, we use the Kalman filter with exact diffuse initial conditions \citep{koopman2000fast,durbin2012time} to compute the log-likelihood of the model. Finally, we used the priors in \cite{hasenzagl2018model}.

\vspace{1em}
\begin{algorithmcustom}[H]{\bfseries Adaptive Metropolis-Within-Gibbs}\label{algo:AMWG}

		\begin{itemize}[]
			\item \textsf{Initialisation} 

			Let $\mathscr{K} \defeq \{1, \ldots, n_k\}$ and denote as $\vect{P}(\mathscr{K})$ a function that returns a random permutation of $\mathscr{K}$ (uniformly taken from the full set of permutations of $\mathscr{K}$). Let also $\vect{\theta}_{0}$ be a $n_k$ dimensional vector corresponding to the initial value for the Metropolis parameters. This vector is associated to a high posterior mass.
			
			\item \textsf{Single component adaptive metropolis} \vspace{0.5em}
			
			\textbf{let} $m=1$ \vspace{0.5em}			
			
			\textbf{for} $j = 1, \ldots , 10000$ \vspace{0.5em}
			
				\hspace{1em} \textbf{let} $\vect{S}_{j} = \vect{P}(\mathscr{K})$ \vspace{0.5em}
			
				\hspace{1em} \textbf{for each} $k$ in $\vect{S}_{j}$
				
				\begin{enumerate}[\hspace{2em} 1.]
					\item \emph{Adaptation:} Update the standard deviation of the proposal distribution
					\begin{equation*}
					\sigma_{k, j} = \begin{cases}
					1 & \text{if } j \leq 10, \\
					\exp\big(\alpha_{k,j-1}-0.44\big) \sigma_{k,j-1} & \text{otherwise},
					\end{cases}
					\end{equation*}
					
					where $\alpha_{k, j-1}$ is the acceptance rate for the iteration $j-1$, for the parameter at position $S_{k,j}$. Besides, $44\%$ is the standard target acceptance rate for single component Metropolis algorithms. \vspace{0.5em}
					
					\item \emph{New candidate:} Generate a candidate vector of parameters $\vect{\theta}^{\,*}_{m}$ such that
					\begin{equation*}
					\theta_{l,m}^{\,*} = \begin{cases}
					\theta_{l,m-1} & \text{if } l \neq k, \\
					\underline{\theta} \iidN \big(\theta_{l,m-1}, \sigma_{k,j} \big) & \text{otherwise},
					\end{cases}
					\end{equation*}
					
					\noindent for $l=1,\ldots,n_k$.
					
					\item \emph{Accept-reject:} Set 
					\begin{equation*}
					\vect{\theta}_{m} =\begin{cases}
					\vect{\theta}^{\,*}_{m} &\text{accept with probability } \eta_{\,m}, \\ 
					\vect{\theta}_{m-1} &\text{reject with probability } 1-\eta_{\,m},
					\end{cases}
					\end{equation*} 
					
					where
					\begin{equation*}
					\eta_{\,m} \defeq \min\left(1, \frac{\vphantom{\Big(}p\,\big[\vect{Y} \mid \vect{f}(\vect{\theta}^{\,*}_{m})^{-1}\big] \, p\,\big[\vect{f}(\vect{\theta}^{\,*}_{m})^{-1}\big] \, J(\vect{\theta}^{\,*}_{m})}{\vphantom{\Big(}p\,\big[\vect{Y} \mid f(\vect{\theta}_{m-1})^{-1}\big] \, p\,\big[\vect{f}(\vect{\theta}_{m-1})^{-1}\big] \, J\big[\vect{\theta}_{m-1}\big]}\right),
					\end{equation*}

					$\vect{f}$ and $J$ are defined below.

					\item \emph{Increase counter:} Increase $m$ by one.
				\end{enumerate}
			
			\item {\bf Gibbs sampling} 
			
			For $j>5000$ (burn-in period), use the univariate approach for multivariate time series of \cite{koopman2000fast} to the simulation smoother proposed in \cite{durbin2002simple} to sample the unobserved states, conditional on the parameters. In doing so, we follow the refinement proposed in \cite{jarocinski2015note}.
		
			\item \textsf{Burn-in period}
			
			Discard the output of the first $j = 1, \ldots , 5000$ iterations.
			
			\item {\bf Jacobian}
			
			As in \cite{hasenzagl2018model} most parameters are bounded in their support (e.g. the variance parameters must be larger than zero). In order to deal with this complexity, this manuscript transforms the bounded parameters ($\vect{\Theta}$) so that the support of the transformed parameters ($\vect{\theta}$) is unbounded. Indeed, the Adaptive Metropolis-Within-Gibbs draws the model parameters in the unbounded space. At a generic iteration $j$, the following transformations have been applied to a generic parameter $i$ with a Normal, Inverse-Gamma or Uniform prior:
			\begin{alignat*}{2}
				&\theta_{i,j}^N &&= \Theta_{i,j}^N  \\[5pt]
				&\theta_{i,j}^{IG} &&= \ln (\Theta_{i,j}^{IG} - a_{i}) \\[5pt]
				&\theta_{i,j}^U &&= \ln \left(\frac{\Theta_{i,j}^U - a_{i}}{b_{i} - \Theta_{i,j}^U}\right),
			\end{alignat*}
			
			\noindent where $a_{i}$ and $b_{i}$ are the lower and the upper bounds for the $i$-th parameter. These transformations are functions $f(\Theta) = \theta$, with inverses $f(\theta)^{-1} = \Theta$ given by:
			\begin{alignat*}{3}
				&\Theta_{i,j}^N = \theta_{i,j}^N \\[5pt]
				&\Theta_{i,j}^{IG} = \exp (\theta_{i,j}^{IG}) + a_{i} \\[5pt]
				&\Theta_{i,j}^{\,U} = \frac{a_{i} + b_{i} \, \exp (\theta_{i,j}^{\,U})}{1+\exp (\theta_{i,j}^{\,U})}.
			\end{alignat*}
			
			\noindent These transformations must be taken into account when evaluating the natural logarithm of the prior densities by adding the Jacobians of the transformations of the variables:
			\begin{alignat*}{3}
				&\ln \left(\frac{d \Theta_{i,j}^N}{d \theta_{i,j}^N}\right) = 0 \\[5pt]
				&\ln \left(\frac{d \Theta_{i,j}^{IG}}{d \theta_{i,j}^{IG}}\right) = \theta_{i,j}^{IG} \\[5pt]
				&\ln \left(\frac{d \Theta_{i,j}^U}{d \theta_{i,j}^U}\right) = \ln (b_{i} - a_{i}) + \theta_{i,j}^U - 2 \ln (1+\exp(\theta_{i,j}^U)).
			\end{alignat*}        
			
		\end{itemize}
\end{algorithmcustom}
\clearpage

\section{Additional Real-Time Results}

\begin{table}[]
\resizebox{\textwidth}{!}{\begin{tabular}{lcccc}
\hline
                                                                 & \multicolumn{2}{c}{Output Gap}      & \multicolumn{2}{c}{Potential Output} \\
                                                                 & Undisciplined & Tracking & Undisciplined & Tracking \\ \hline
Mean of std dev & 0.54               & 0.61           & 6.79                & 8.33           \\
Mean of std dev (until 2005) & 0.5                & 0.5            & 5.06                & 7.28           \\
Mean of max revision     & 0.91               & 1.37           & 16.38               & 15.09          \\
Mean of max revision (until 2005)    & 0.46               & 1.13           & 9.10                & 10.93 \\ \hline         
\end{tabular}}
\caption{The first two rows of this table report the standard deviation of the output gap and potential output computed across vintages for each reference month and then averaged across reference months. The last two columns report the maximum absolute value of revisions computed for each reference month and then averaged across reference months.}
\label{tab:revisions_statistics}
\end{table}

\begin{figure}[htbp]
	\centering
	\includegraphics[width=\textwidth]{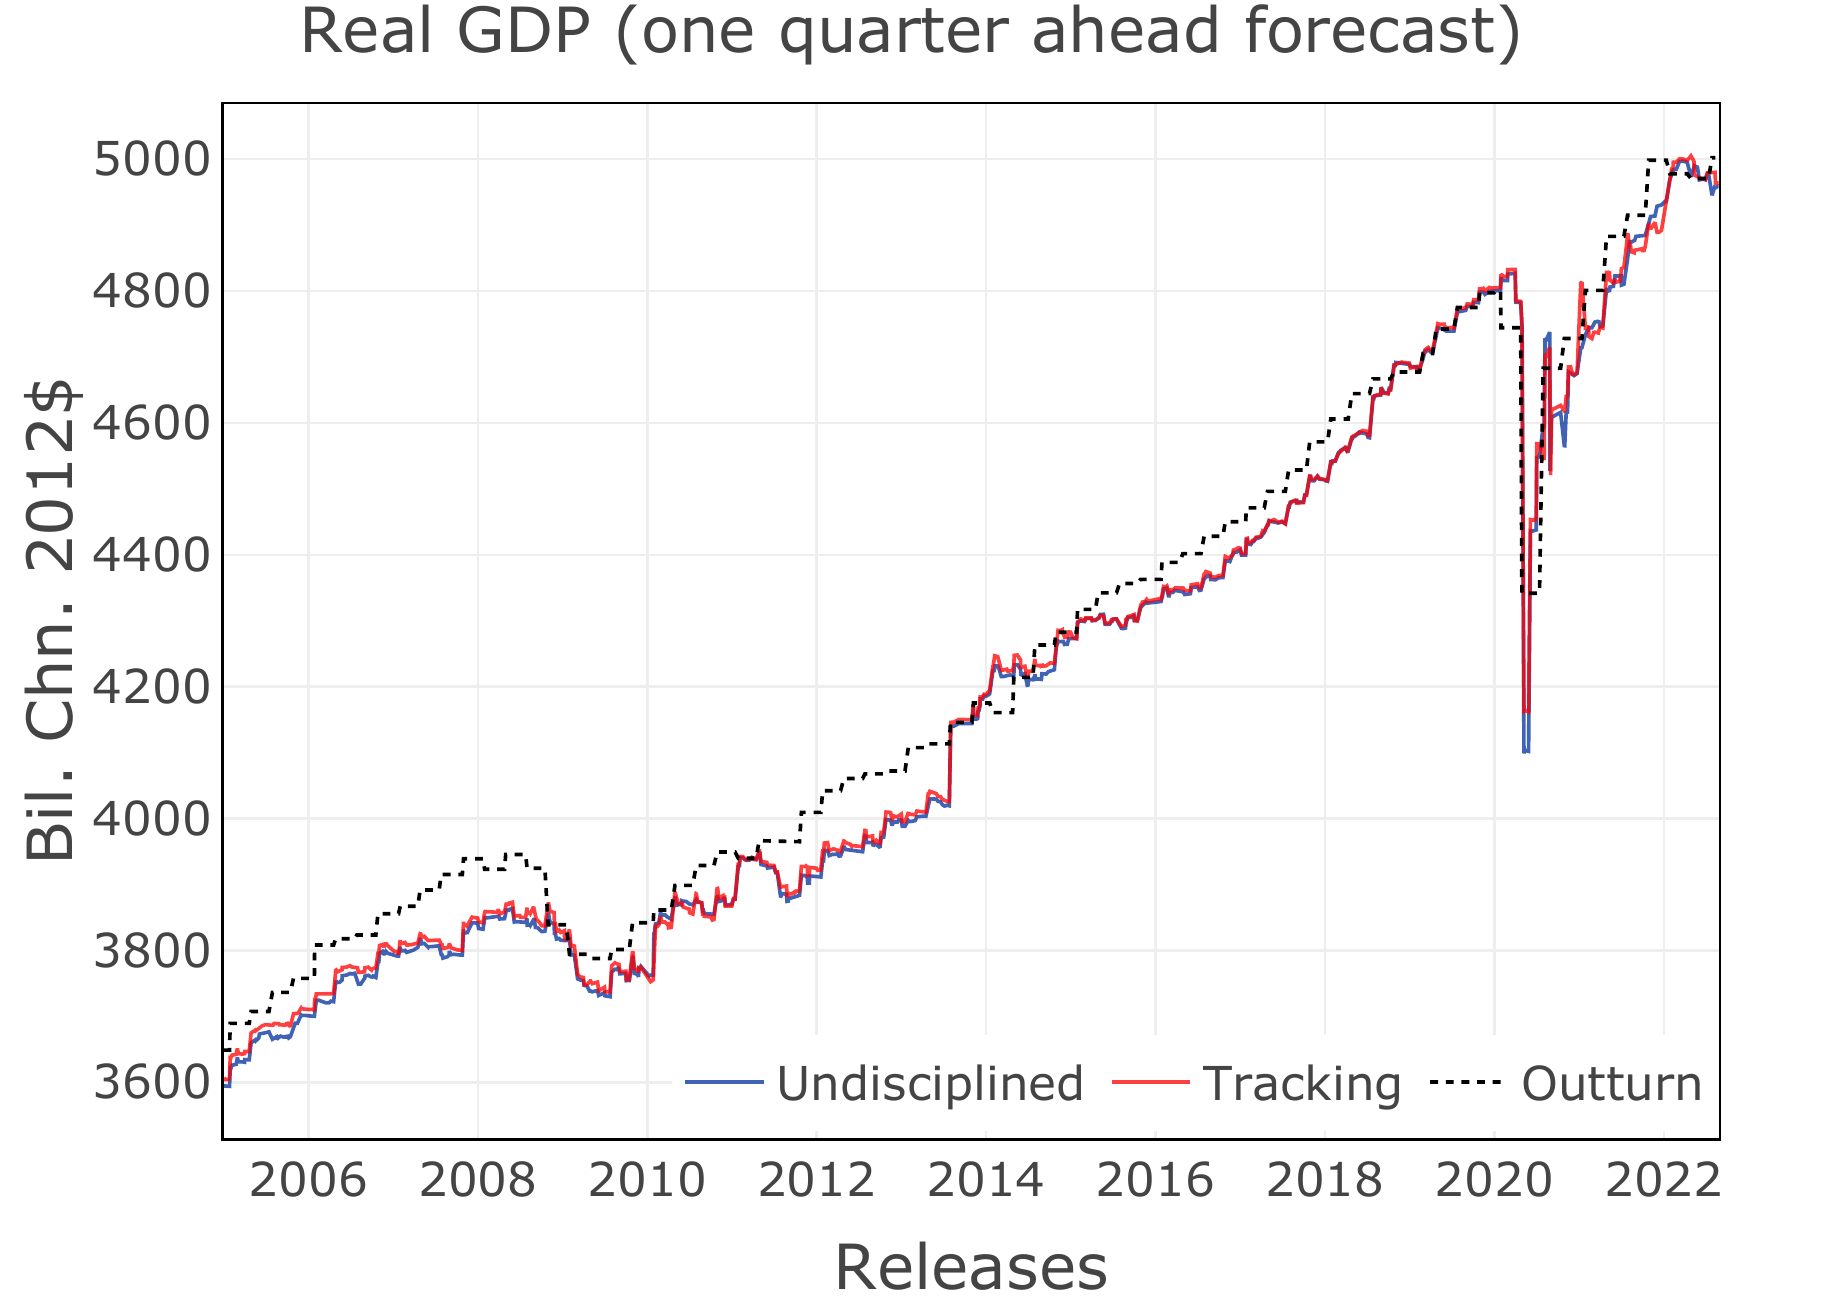}
	\caption{The chart reports the one quarter ahead, real time forecasts of Real GDP from the two models and compares them to the outturn. The out-of-sample evaluation starts in Jan-2005 and ends in Sept-2020.}
\end{figure}

\begin{figure}[htbp]
	\centering
	\includegraphics[width=\textwidth]{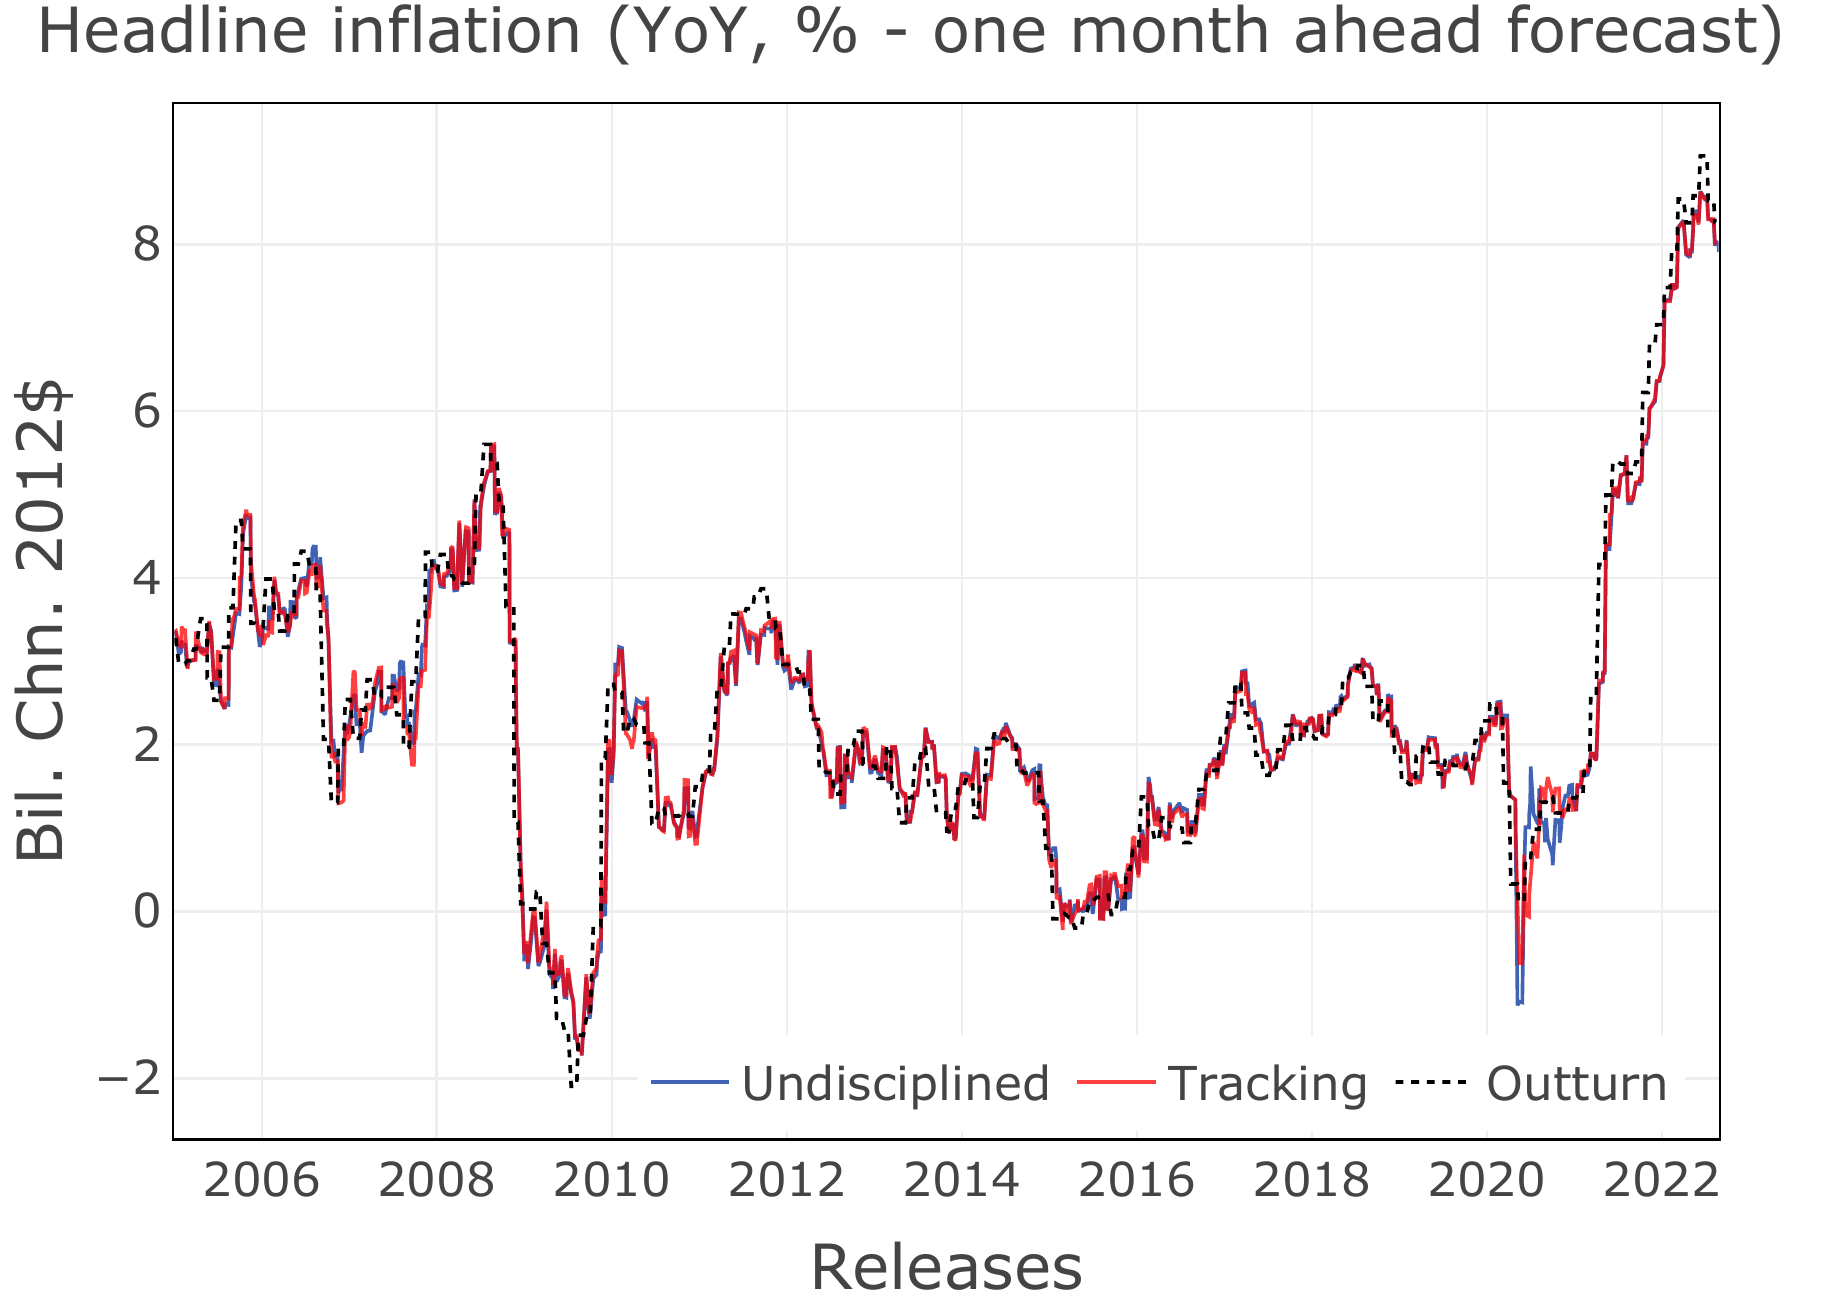}
	\caption{The chart reports the one month ahead, real time forecasts of inflation from the two models and compares them to the outturn. The out-of-sample evaluation starts in Jan-2005 and ends in Sept-2020.}
\end{figure}

\begin{figure}[htbp]
	\centering
	\includegraphics[width=\textwidth]{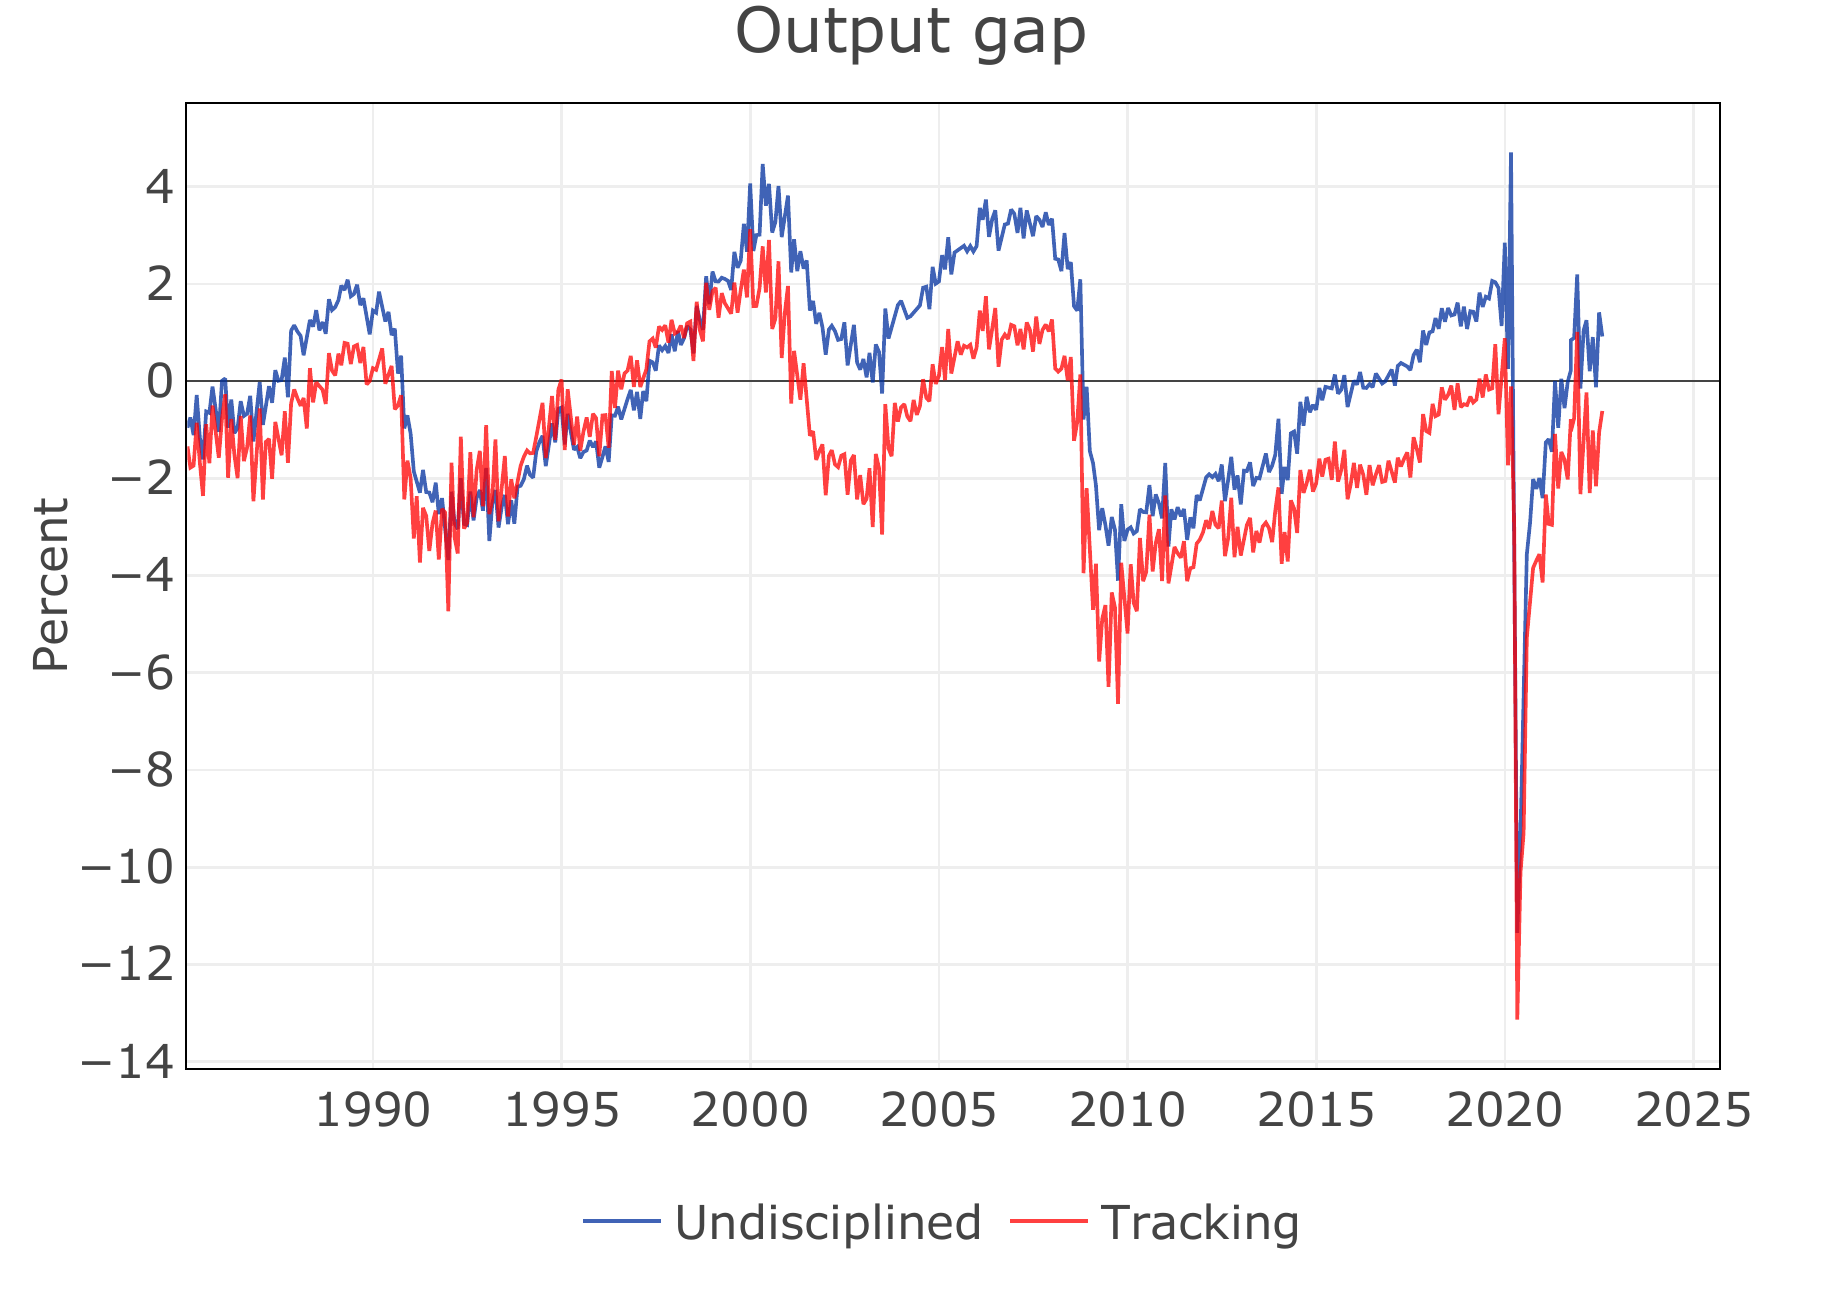}
	\caption{The chart compares the output gap estimates from the two models computed using the final (09/30/2020) data vintage from the out-of-sample forecasting exercise.}
\end{figure}

%\begin{figure}[htbp]
%	\centering
%	\includegraphics[width=\textwidth]{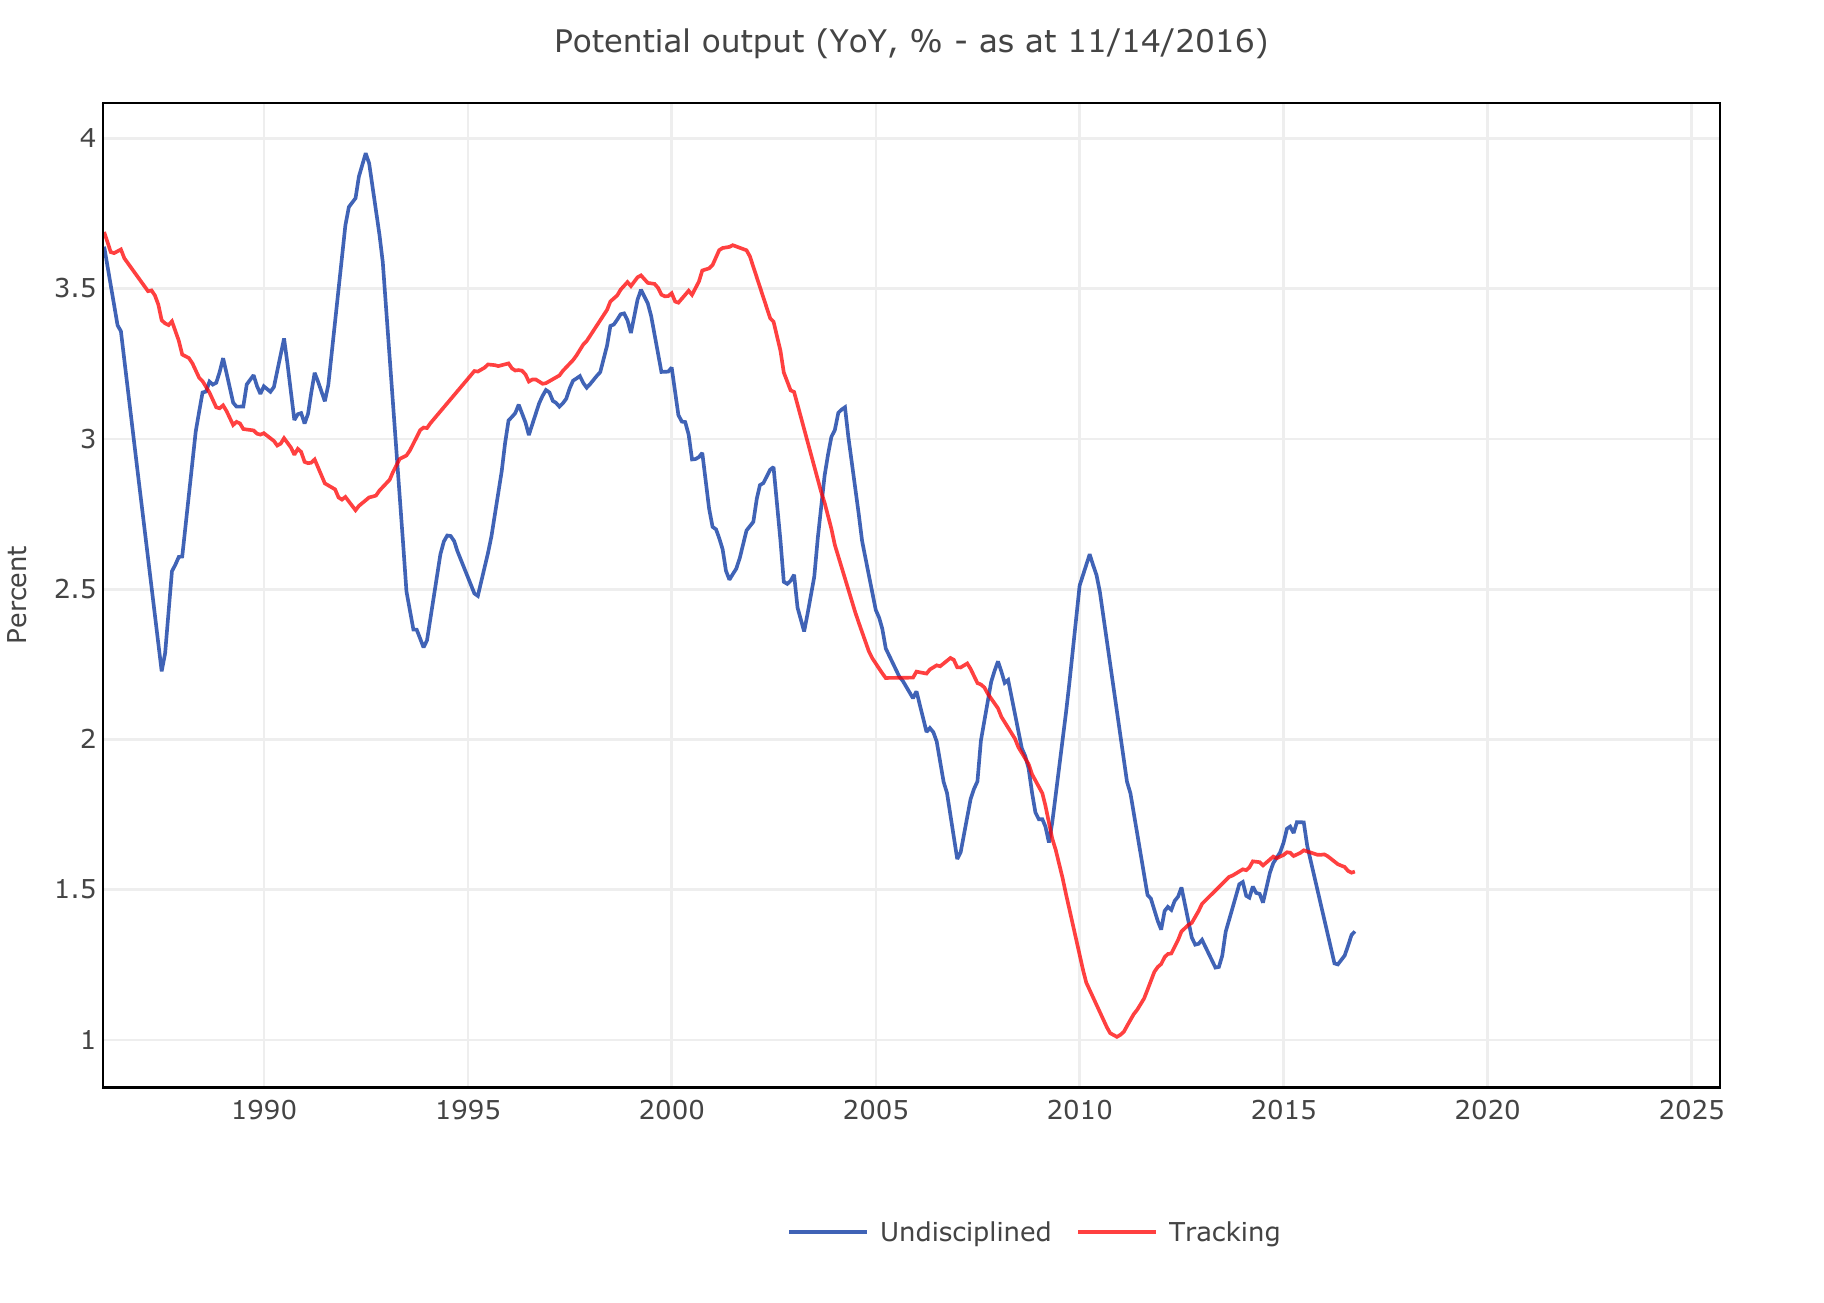}
%	\caption{The chart compares the year-on-year growth rates of potential GDP from the two models computed using the final (09/30/2020) data vintage from the out-of-sample forecasting exercise.}
%	\label{fig:potential_yoy}
%\end{figure}

\end{appendices}
